# Supplementary material for: Ultrafast Photochemistry and Electron Diffraction for Cyclobutanone in the S2 State: Surface Hopping with Time-Dependent Density Functional Theory
Source: arXiv:2402.10336 ancillary file (2024-02-15)
Supplement: Supplementary file 1 [file supplement.pdf]

Supplemental Information for

# Ultrafast Photochemistry and Electron Diffraction for Cyclobutanone in the $S_2$ State: Surface Hopping with Time-Dependent Density Functional Theory

Ericka Roy Miller, Sean Hoehn, Abhijith Kumar, Dehua Jiang, and Shane M. Parker[a)]
*Department of Chemistry, Case Western Reserve University*
*10900 Euclid Ave, Cleveland, OH 44106, USA*

This supplemental information is organized as follows:

- Section I: Details on the outcomes of individual PBE0-FSSH trajectories
- Section II: Details on UED simulation and additional figures for selected structures
- Section III: Full data set for Landau-Zener ISC probabilties

[a)]Electronic mail: shane.parker@case.edu

## I. PBE0-FSSH TRAJECTORY OUTCOME STATISTICS

TABLE SI: Trajectory outcome statistics and details for PBE0-FSSH trajectories 0 through 49

| Trajectory | S2→S1 Hop (ps) | S2→S1 CI | S1→S0 Hop (ps) | S1→S0 CI | Final State | Dissociation Products |
|---|---|---|---|---|---|---|
| 0 | 4.115 | CH stretch | 4.388 | $\alpha$ stretch | 0 | none |
| 1 | 6.713 | CH stretch | 7.112 | $\alpha$ stretch | 0 | none |
| 2 | 0.128 | $\beta$ stretch | 0.486 | $\alpha$ stretch | 0 | none |
| 3 | 2.953 | CH stretch | 3.514 | $\alpha$ stretch | 0 | none |
| 4 | n/a | n/a | n/a | n/a | 2 | none |
| 5 | 8.894 | CH stretch | 9.152 | $\alpha$ stretch | 0 | none |
| 6 | 8.439 | CH stretch | n/a | n/a | 1 | none |
| 7 | 7.805 | CH stretch | 9.049 | $\alpha$ stretch | 0 | none |
| 8 | 6.128 | $\beta$ stretch | 6.637 | $\alpha$ stretch | 0 | C2 |
| 9 | 0.022 | $\beta$ stretch | 0.101 | $\alpha$ stretch | 0 | C2 |
| 10 | 8.902 | CH stretch | n/a | n/a | 1 | none |
| 11 | 7.829 | CH stretch | 9.532 | $\alpha$ stretch | 0 | none |
| 12 | 0.104 | $\beta$ stretch | 0.900 | $\alpha$ stretch | 0 | none |
| 13 | 5.787 | CH stretch | 5.942 | $\alpha$ stretch | 0 | none |
| 14 | n/a | n/a | n/a | n/a | 2 | none |
| 15 | 4.262 | CH stretch | 4.479 | $\alpha$ stretch | 0 | none |
| 16 | 4.562 | CH stretch | 5.234 | $\alpha$ stretch | 0 | none |
| 17 | 5.507 | CH stretch | 6.048 | $\alpha$ stretch | 0 | none |
| 18 | 5.852 | CH stretch | 6.136 | $\alpha$ stretch | 0 | none |
| 19 | n/a | n/a | n/a | n/a | 2 | none |
| 20 | 8.497 | CH stretch | 9.200 | $\alpha$ stretch | 0 | none |
| 21 | 4.673 | CH stretch | 4.878 | $\alpha$ stretch | 0 | none |
| 22 | 6.242 | CH stretch | 7.001 | $\alpha$ stretch | 0 | none |
| 23 | n/a | n/a | n/a | n/a | 2 | none |
| 24 | 5.139 | CH stretch | 5.313 | $\alpha$ stretch | 0 | none |
| 25 | 3.024 | CH stretch | 3.537 | $\alpha$ stretch | 0 | none |
| 26 | 1.629 | CH stretch | 1.759 | $\alpha$ stretch | 0 | none |
| 27 | n/a | n/a | n/a | n/a | 2 | none |
| 28 | 3.120 | CH stretch | 3.451 | no conv | 0 | none |
| 29 | n/a | n/a | n/a | n/a | 2 | none |
| 30 | 2.617 | CH stretch | 4.367 | $\alpha$ stretch | 0 | none |
| 31 | 4.253 | CH stretch | 4.801 | $\alpha$ stretch | 0 | none |
| 32 | 0.083 | $\beta$ stretch | 0.103 | $\alpha$ stretch | 0 | none |
| 33 | 0.051 | $\beta$ stretch | 0.068 | $\alpha$ stretch | 0 | none |
| 34 | n/a | n/a | n/a | n/a | 2 | none |
| 35 | n/a | n/a | n/a | n/a | 2 | none |
| 36 | 4.894 | CH stretch | 5.115 | no conv | 0 | none |
| 37 | 6.604 | CH stretch | 7.163 | $\alpha$ stretch | 0 | none |
| 38 | 1.565 | CH stretch | 2.016 | $\alpha$ stretch | 0 | none |
| 39 | 0.122 | $\beta$ stretch | 0.145 | $\alpha$ stretch | 0 | C2 |
| 40 | 0.622 | $\beta$ stretch | 1.723 | $\alpha$ stretch | 0 | none |
| 41 | 2.440 | $\beta$ stretch | 2.862 | $\alpha$ stretch | 0 | none |
| 42 | 2.143 | CH stretch | 2.818 | $\alpha$ stretch | 0 | none |
| 43 | n/a | n/a | n/a | n/a | 2 | none |
| 44 | 7.648 | CH stretch | 8.456 | $\alpha$ stretch | 0 | none |
| 45 | 2.619 | CH stretch | 3.943 | $\alpha$ stretch | 0 | none |
| 46 | 0.018 | $\beta$ stretch | 1.477 | $\alpha$ stretch | 0 | none |
| 47 | 4.607 | CH stretch | 5.072 | $\alpha$ stretch | 0 | none |
| 48 | 3.776 | CH stretch | 4.733 | $\alpha$ stretch | 0 | none |
| 49 | 3.429 | CH stretch | 4.426 | $\alpha$ stretch | 0 | none |

TABLE SII: Trajectory outcome statistics and details for PBE0-FSSH trajectories 50 through 99

| Trajectory | S2→S1 Hop (ps) | S2→S1 CI | S1→S0 Hop (ps) | S1→S0 CI | Final State | Dissociation Products |
|---|---|---|---|---|---|---|
| 50 | 0.028 | $\beta$ stretch | 0.318 | $\alpha$ stretch | 0 | C2 |
| 51[1] | 2.323 | other | n/a | n/a | 0 | none |
| 52 | 2.335 | $\beta$ stretch | 2.411 | no conv | 0 | none |
| 53 | 0.016 | $\beta$ stretch | 0.790 | $\alpha$ stretch | 0 | none |
| 54 | 9.132 | CH stretch | n/a | n/a | 1 | none |
| 55 | 2.654 | CH stretch | 2.803 | $\alpha$ stretch | 0 | C2 |
| 56 | 0.481 | CH stretch | 0.996 | $\alpha$ stretch | 0 | none |
| 57 | 1.609 | CH stretch | 1.781 | $\alpha$ stretch | 0 | none |
| 58 | 0.754 | CH stretch | 1.615 | $\alpha$ stretch | 0 | none |
| 59 | n/a | n/a | n/a | n/a | 2 | none |
| 60 | 2.898 | CH stretch | 3.633 | $\alpha$ stretch | 0 | none |
| 61 | n/a | n/a | n/a | n/a | 2 | none |
| 62 | 4.335 | CH stretch | 4.877 | $\alpha$ stretch | 0 | none |
| 63 | 2.841 | CH stretch | 3.827 | $\alpha$ stretch | 0 | none |
| 64 | n/a | n/a | n/a | n/a | 2 | none |
| 65[2] | 0.933 | $\beta$ stretch | n/a | n/a | 0 | none |
| 66 | 6.188 | CH stretch | 6.429 | $\alpha$ stretch | 0 | none |
| 67 | 5.734 | CH stretch | 5.825 | $\alpha$ stretch | 0 | none |
| 68 | 6.740 | CH stretch | 6.890 | $\alpha$ stretch | 0 | none |
| 69 | n/a | n/a | n/a | n/a | 2 | none |
| 70 | 9.070 | CH stretch | n/a | n/a | 1 | none |
| 71 | n/a | n/a | n/a | n/a | 2 | none |
| 72 | 7.279 | CH stretch | 7.934 | $\alpha$ stretch | 0 | none |
| 73 | 0.903 | CH stretch | 0.995 | $\alpha$ stretch | 0 | none |
| 74 | 0.936 | CH stretch | 1.785 | $\alpha$ stretch | 0 | none |
| 75 | 7.335 | CH stretch | 7.467 | $\alpha$ stretch | 0 | none |
| 76 | n/a | n/a | n/a | n/a | 2 | none |
| 77 | 3.348 | CH stretch | 3.801 | other | 0 | none |
| 78 | 0.766 | other | 2.029 | $\alpha$ stretch | 0 | none |
| 79 | 1.801 | CH stretch | 2.133 | $\alpha$ stretch | 0 | none |
| 80 | 4.984 | CH stretch | 6.307 | $\alpha$ stretch | 0 | none |
| 81 | 9.085 | CH stretch | 9.461 | $\alpha$ stretch | 0 | none |
| 82 | 9.632 | CH stretch | n/a | n/a | 1 | none |
| 83 | n/a | n/a | n/a | n/a | 2 | none |
| 84 | 8.652 | CH stretch | 8.811 | $\alpha$ stretch | 0 | none |
| 85 | 1.639 | CH stretch | 2.630 | $\alpha$ stretch | 0 | C2 |
| 86 | 3.990 | CH stretch | 4.181 | $\alpha$ stretch | 0 | none |
| 87 | 6.494 | CH stretch | 6.754 | $\alpha$ stretch | 0 | none |
| 88 | 5.321 | CH stretch | 6.098 | $\alpha$ stretch | 0 | none |
| 89 | n/a | n/a | n/a | n/a | 2 | none |
| 90 | 4.408 | CH stretch | 5.521 | $\alpha$ stretch | 0 | C3 |
| 91 | 7.134 | CH stretch | 7.758 | $\alpha$ stretch | 0 | none |
| 92 | 3.611 | CH stretch | 4.311 | $\alpha$ stretch | 0 | none |
| 93 | 7.124 | CH stretch | 7.985 | $\alpha$ stretch | 0 | none |
| 94 | 1.469 | CH stretch | 1.758 | $\alpha$ stretch | 0 | C2 |
| 95 | 5.703 | CH stretch | 5.958 | $\alpha$ stretch | 0 | none |
| 96 | 0.067 | $\beta$ stretch | 0.186 | $\alpha$ stretch | 0 | C2 |
| 97 | 1.038 | CH stretch | 1.217 | $\alpha$ stretch | 0 | none |
| 98 | 4.501 | CH stretch | 5.062 | $\alpha$ stretch | 0 | none |
| 99 | 6.049 | CH stretch | 6.490 | $\alpha$ stretch | 0 | none |

## II. SIMULATION OF ELECTRON DIFFRACTION SPECTRA

The Ultrafast Electron Diffraction (UED) spectra for the cyclobutanone molecule was simulated based on the Independent Atom Model (IAM).[3] All simulations utilized the code developed by Thomas J.A. Wolf.[4] According to IAM, each atom is considered as a lone scatterer and it assumes that the molecule is a set of non interacting atoms.Thus, this model helps us to consider the elastic scattering amplitude of individual atoms. The elastic scattering amplitude of an individual atom is given by the Mott-Bethe equation

$$f(s) = \frac{me^2}{2\pi\varepsilon_0 h^2}\frac{1}{s^2}[Z - F(s)] = \frac{2}{a_0 s^2}[Z - F(s)], \tag{1}$$

where $f(s)$ represents the atomic form factor (AFF) of electron scattering. AFF is a measure of the elastic scattering amplitude of individual atoms. $s$ is the scattering vector, $m$ is the electron mass, $e$ is the electron charge, $\varepsilon_0$ is the permittivity of free space, $h$ is the Planck constant, $Z$ represents the atomic number, $F(s)$ is the AFF of X-ray scattering,and $a_0$ is the Bohr radius. The elastic electron scattering AFF for each atom was computed using the ELSEPA program.[5] The elastic scattering amplitude of a molecule with N atoms is given by

$$f_{\mathrm{M}}(s) = \sum_{i=1}^{N} f_i(s)e^{is\cdot\boldsymbol{r}_i} \tag{2}$$

where $f_{\mathrm{M}}(s)$ is the molecular structure factor, $f_i(s)$ is the electron scattering atomic form factor of the $i$-th atom. $s$ is the scattering vector, $r_i$ is the position vector of the $i$-th atom. $e^{is\cdot\boldsymbol{r}_i}$ is the phase factor due to the position of the atom.

The total elastic scattering intensity $I_s$ for a molecule can be written as sum of atomic scattering intensity $I_{\mathrm{at}}$ and molecular scattering intensity $I_{\mathrm{mol}}$.

$$I_s = I_{at} + I_{mol} = \sum_{i=1}^{N} |f_i(s)|^2 + \sum_{i=1}^{N}\sum_{\substack{j=1\\ j\neq i}}^{N} f_i^*(s)f_j(s)\frac{\sin(sr_{ij})}{sr_{ij}} \tag{3}$$

where $r_{ij}$ is the interatomic distance. During the entire calculations the range of s values was choosen from 0 to 12 $\text{Å}^{-1}$. The atomic scattering intensity accounts for the scattering amplitudes of individual atoms, while molecular scattering intensity accounts for the combined effect of the scattering amplitudes of all the atoms in the molecule. We then computed the modified scattering intensity from the $I_{atm}$ and $I_{mol}$, and we did the calculations of static ($PDF(R)$) and difference pair distribution functions ($\Delta PDF$) from the modified scattering intensity. The modified scattering intensity $sM(s)$, was calculated and is given by

$$sM(s) = s\frac{I_{mol}}{I_{atm}} \tag{4}$$

Then, a Fourier transform of the $sM(s)$ was performed to obtain the $PDF(R)$

$$PDF(R) = \int_0^{s_{max}} sM(s)\sin(sR)e^{-ks^2}\,ds \tag{5}$$

where $s_{max}$ is the maximum scattering vector, $R$ is the interatomic distance, and $k = 0.03$ was choosen as a damping factor.

Inorder to compute the difference pair distribution function $\Delta PDF(R,t)$, we calculated $\Delta sM(s,t)$. The $\Delta sM(s,t)$ was calculated as

$$\Delta sM(s,t) = s\frac{I_{mol}(s,t) - I_{mol}(s,o)}{I_{at}(s)} \tag{6}$$

where $I_{mol}(s,t)$ is the average molecular scattering intensity at time $t$ across all NAMD trajectories, $I_{mol}(s,0)$ is the average molecular scattering intensity at time 0 across all trajectories, and $I_{at}(s)$ is the atomic scattering intensity. The $\Delta PDF(R,t)$ was then calculated by performing a Fourier transform of the $\Delta sM(s,t)$ and is given by

$$\Delta PDF(R,t) = \int_0^{s_{max}} \Delta sM(s,t)\sin(sR)e^{-ks^2}\,ds \tag{7}$$

To match with the experimental results, we then applied a Gaussian convolution of FWHM = 150 fs on the $\Delta PDF(R,t)$.

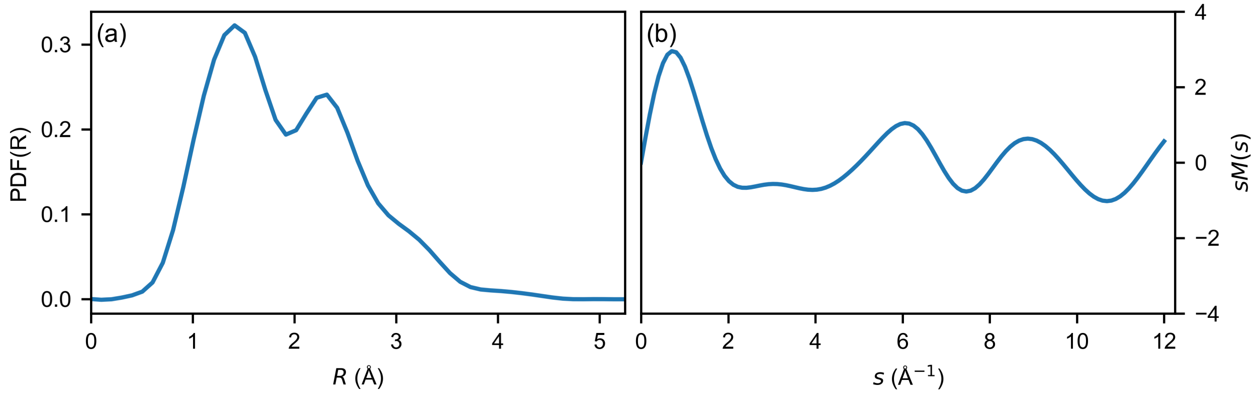


FIG. S1: PDF(R) and sM(s) plots of $S_0$ optimized cyclobutanone

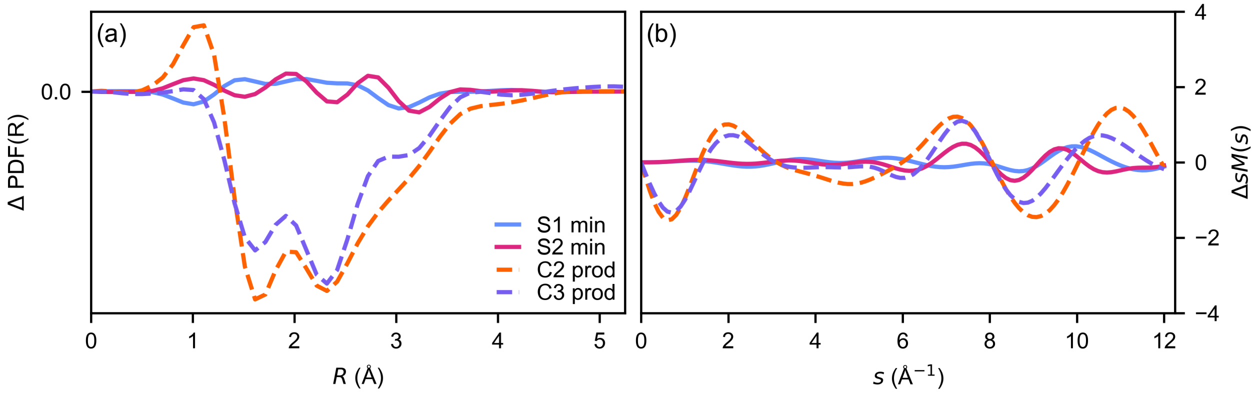


FIG. S2: Δ PDF(R) and Δ sM(s) plots of selected structures with reference to $S_0$ optimized cyclobutanone

[1]Directly hopped from $S_2$ to $S_0$.
[2]Directly hopped from $S_2$ to $S_0$.

[3]M. Centurion, T. J. Wolf, and J. Yang, "Ultrafast imaging of molecules with electron diffraction," Annu. Rev. Phys. Chem. **73**, 21–42 (2022).
[4]T. J. A. Wolf, "Diffraction simulation," `https://github.com/ThomasJAWolf/Diffraction_simulation` (2020).
[5]F. Salvat, A. Jablonski, and C. J. Powell, "Elsepa—dirac partial-wave calculation of elastic scattering of electrons and positrons by atoms, positive ions and molecules," Computer physics communications **165**, 157–190 (2005).

## III. ADDITIONAL DATA FROM LANDAU-ZENER ANALYSIS

TABLE SIII: Landau-Zener probabilities calculated using root-mean-square (RMS) of the energy gaps and spin-orbit couplings between each pair of singlet and triplet.

| Tn | Sn | job11 | job14 | job36 | job54 | job66 | job67 | job7 | job87 | job90 | average |
|---|---|---|---|---|---|---|---|---|---|---|---|
| 0 | 0 | $3.669\times10^{-4}$ | $2.797\times10^{-4}$ | $2.669\times10^{-4}$ | $2.477\times10^{-4}$ | $2.351\times10^{-4}$ | $2.544\times10^{-4}$ | $3.937\times10^{-4}$ | $2.525\times10^{-4}$ | $1.761\times10^{-4}$ | $2.748\times10^{-4}$ |
| 1 | 0 | $3.371\times10^{-3}$ | $3.681\times10^{-3}$ | $1.562\times10^{-3}$ | $3.630\times10^{-3}$ | $1.783\times10^{-3}$ | $1.498\times10^{-3}$ | $2.742\times10^{-3}$ | $1.645\times10^{-3}$ | $8.852\times10^{-4}$ | $2.311\times10^{-3}$ |
| 2 | 0 | $2.156\times10^{-3}$ | $4.199\times10^{-3}$ | $1.598\times10^{-3}$ | $3.032\times10^{-3}$ | $1.997\times10^{-3}$ | $1.629\times10^{-3}$ | $3.018\times10^{-3}$ | $1.653\times10^{-3}$ | $8.347\times10^{-4}$ | $2.235\times10^{-3}$ |
| 3 | 0 | $8.622\times10^{-4}$ | $9.972\times10^{-4}$ | $5.483\times10^{-4}$ | $9.443\times10^{-4}$ | $5.809\times10^{-4}$ | $5.263\times10^{-4}$ | $7.574\times10^{-4}$ | $5.797\times10^{-4}$ | $1.677\times10^{-4}$ | $6.627\times10^{-4}$ |
| 4 | 0 | $7.236\times10^{-4}$ | $8.190\times10^{-4}$ | $3.934\times10^{-4}$ | $7.393\times10^{-4}$ | $4.276\times10^{-4}$ | $3.774\times10^{-4}$ | $6.741\times10^{-4}$ | $4.511\times10^{-4}$ | $1.092\times10^{-4}$ | $5.239\times10^{-4}$ |
| 0 | 1 | $9.703\times10^{-4}$ | $7.064\times10^{-4}$ | $1.490\times10^{-3}$ | $8.934\times10^{-4}$ | $1.269\times10^{-3}$ | $1.222\times10^{-3}$ | $1.164\times10^{-3}$ | $1.123\times10^{-3}$ | $4.693\times10^{-4}$ | $1.034\times10^{-3}$ |
| 1 | 1 | $2.254\times10^{-4}$ | $9.310\times10^{-5}$ | $8.446\times10^{-5}$ | $1.324\times10^{-4}$ | $1.076\times10^{-4}$ | $9.898\times10^{-5}$ | $1.336\times10^{-4}$ | $1.080\times10^{-4}$ | $4.523\times10^{-5}$ | $1.143\times10^{-4}$ |
| 2 | 1 | $7.173\times10^{-4}$ | $4.188\times10^{-4}$ | $5.584\times10^{-4}$ | $5.492\times10^{-4}$ | $5.247\times10^{-4}$ | $5.199\times10^{-4}$ | $7.576\times10^{-4}$ | $4.471\times10^{-4}$ | $2.325\times10^{-4}$ | $5.251\times10^{-4}$ |
| 3 | 1 | $1.855\times10^{-4}$ | $1.066\times10^{-4}$ | $2.286\times10^{-4}$ | $1.930\times10^{-4}$ | $2.087\times10^{-4}$ | $2.020\times10^{-4}$ | $1.686\times10^{-4}$ | $2.316\times10^{-4}$ | $6.259\times10^{-5}$ | $1.764\times10^{-4}$ |
| 4 | 1 | $1.975\times10^{-4}$ | $1.318\times10^{-4}$ | $1.634\times10^{-4}$ | $1.982\times10^{-4}$ | $1.597\times10^{-4}$ | $1.352\times10^{-4}$ | $1.225\times10^{-4}$ | $1.627\times10^{-4}$ | $4.527\times10^{-5}$ | $1.463\times10^{-4}$ |
| 0 | 2 | $3.884\times10^{-3}$ | $7.623\times10^{-3}$ | $2.151\times10^{-3}$ | $5.746\times10^{-3}$ | $2.936\times10^{-3}$ | $2.153\times10^{-3}$ | $4.536\times10^{-3}$ | $2.288\times10^{-3}$ | $9.552\times10^{-4}$ | $3.586\times10^{-3}$ |
| 1 | 2 | $8.266\times10^{-4}$ | $6.948\times10^{-4}$ | $6.866\times10^{-4}$ | $7.398\times10^{-4}$ | $6.965\times10^{-4}$ | $6.460\times10^{-4}$ | $1.067\times10^{-3}$ | $5.890\times10^{-4}$ | $2.196\times10^{-4}$ | $6.851\times10^{-4}$ |
| 2 | 2 | $2.688\times10^{-4}$ | $2.780\times10^{-4}$ | $1.644\times10^{-4}$ | $2.769\times10^{-4}$ | $1.520\times10^{-4}$ | $1.324\times10^{-4}$ | $1.932\times10^{-4}$ | $1.726\times10^{-4}$ | $3.404\times10^{-5}$ | $1.858\times10^{-4}$ |
| 3 | 2 | $1.098\times10^{-4}$ | $1.979\times10^{-4}$ | $1.199\times10^{-4}$ | $2.236\times10^{-4}$ | $1.497\times10^{-4}$ | $1.090\times10^{-4}$ | $1.617\times10^{-4}$ | $1.383\times10^{-4}$ | $3.292\times10^{-5}$ | $1.381\times10^{-4}$ |
| 4 | 2 | $8.529\times10^{-4}$ | $1.383\times10^{-3}$ | $3.673\times10^{-4}$ | $1.039\times10^{-3}$ | $4.876\times10^{-4}$ | $3.879\times10^{-4}$ | $8.949\times10^{-4}$ | $4.124\times10^{-4}$ | $1.316\times10^{-4}$ | $6.619\times10^{-4}$ |
| 0 | 3 | $4.291\times10^{-4}$ | $3.006\times10^{-4}$ | $3.002\times10^{-4}$ | $3.827\times10^{-4}$ | $3.353\times10^{-4}$ | $2.568\times10^{-4}$ | $3.292\times10^{-4}$ | $3.449\times10^{-4}$ | $1.682\times10^{-4}$ | $3.163\times10^{-4}$ |
| 1 | 3 | $7.704\times10^{-4}$ | $5.790\times10^{-4}$ | $6.675\times10^{-4}$ | $6.693\times10^{-4}$ | $6.943\times10^{-4}$ | $5.230\times10^{-4}$ | $7.103\times10^{-4}$ | $5.762\times10^{-4}$ | $2.047\times10^{-4}$ | $5.994\times10^{-4}$ |
| 2 | 3 | $1.394\times10^{-4}$ | $2.744\times10^{-4}$ | $3.830\times10^{-4}$ | $2.295\times10^{-4}$ | $4.480\times10^{-4}$ | $3.145\times10^{-4}$ | $3.000\times10^{-4}$ | $2.894\times10^{-4}$ | $7.759\times10^{-5}$ | $2.729\times10^{-4}$ |
| 3 | 3 | $1.262\times10^{-4}$ | $6.376\times10^{-5}$ | $2.575\times10^{-4}$ | $1.188\times10^{-4}$ | $2.219\times10^{-4}$ | $1.626\times10^{-4}$ | $1.528\times10^{-4}$ | $1.841\times10^{-4}$ | $3.594\times10^{-5}$ | $1.471\times10^{-4}$ |
| 4 | 3 | $1.927\times10^{-4}$ | $1.394\times10^{-4}$ | $1.433\times10^{-4}$ | $1.518\times10^{-4}$ | $1.468\times10^{-4}$ | $1.144\times10^{-4}$ | $1.509\times10^{-4}$ | $1.409\times10^{-4}$ | $3.718\times10^{-5}$ | $1.353\times10^{-4}$ |
| 0 | 4 | $3.825\times10^{-4}$ | $3.435\times10^{-4}$ | $3.384\times10^{-4}$ | $3.550\times10^{-4}$ | $3.621\times10^{-4}$ | $2.701\times10^{-4}$ | $4.231\times10^{-4}$ | $3.025\times10^{-4}$ | $1.565\times10^{-4}$ | $3.260\times10^{-4}$ |
| 1 | 4 | $2.223\times10^{-3}$ | $2.734\times10^{-3}$ | $1.049\times10^{-3}$ | $2.641\times10^{-3}$ | $1.410\times10^{-3}$ | $9.464\times10^{-4}$ | $1.442\times10^{-3}$ | $1.089\times10^{-3}$ | $4.297\times10^{-4}$ | $1.552\times10^{-3}$ |
| 2 | 4 | $1.126\times10^{-3}$ | $2.813\times10^{-3}$ | $1.163\times10^{-3}$ | $1.932\times10^{-3}$ | $1.630\times10^{-3}$ | $1.295\times10^{-3}$ | $1.826\times10^{-3}$ | $1.223\times10^{-3}$ | $3.405\times10^{-4}$ | $1.483\times10^{-3}$ |
| 3 | 4 | $2.929\times10^{-4}$ | $2.199\times10^{-4}$ | $5.058\times10^{-4}$ | $2.772\times10^{-4}$ | $5.515\times10^{-4}$ | $4.044\times10^{-4}$ | $3.610\times10^{-4}$ | $4.202\times10^{-4}$ | $7.435\times10^{-5}$ | $3.453\times10^{-4}$ |
| 4 | 4 | $5.052\times10^{-4}$ | $4.969\times10^{-4}$ | $4.235\times10^{-4}$ | $4.866\times10^{-4}$ | $4.608\times10^{-4}$ | $3.739\times10^{-4}$ | $5.355\times10^{-4}$ | $4.367\times10^{-4}$ | $9.903\times10^{-5}$ | $4.242\times10^{-4}$ |
| 0 | 5 | $3.619\times10^{-4}$ | $4.862\times10^{-4}$ | $3.999\times10^{-4}$ | $4.439\times10^{-4}$ | $4.229\times10^{-4}$ | $3.363\times10^{-4}$ | $3.947\times10^{-4}$ | $3.898\times10^{-4}$ | $1.444\times10^{-4}$ | $3.756\times10^{-4}$ |
| 1 | 5 | $1.640\times10^{-3}$ | $1.680\times10^{-3}$ | $8.967\times10^{-4}$ | $1.840\times10^{-3}$ | $1.107\times10^{-3}$ | $7.967\times10^{-4}$ | $1.240\times10^{-3}$ | $8.765\times10^{-4}$ | $3.285\times10^{-4}$ | $1.156\times10^{-3}$ |
| 2 | 5 | $2.028\times10^{-3}$ | $5.838\times10^{-3}$ | $1.982\times10^{-3}$ | $4.464\times10^{-3}$ | $2.732\times10^{-3}$ | $2.044\times10^{-3}$ | $3.817\times10^{-3}$ | $2.285\times10^{-3}$ | $6.201\times10^{-4}$ | $2.868\times10^{-3}$ |
| 3 | 5 | $3.904\times10^{-4}$ | $4.979\times10^{-4}$ | $6.641\times10^{-4}$ | $7.023\times10^{-4}$ | $6.682\times10^{-4}$ | $5.961\times10^{-4}$ | $4.922\times10^{-4}$ | $7.114\times10^{-4}$ | $1.232\times10^{-4}$ | $5.384\times10^{-4}$ |
| 4 | 5 | $6.901\times10^{-4}$ | $1.312\times10^{-3}$ | $6.970\times10^{-4}$ | $1.024\times10^{-3}$ | $7.139\times10^{-4}$ | $6.383\times10^{-4}$ | $8.469\times10^{-4}$ | $8.245\times10^{-4}$ | $1.196\times10^{-4}$ | $7.629\times10^{-4}$ |

TABLE SIV: Landau-Zener probabilities calculated using root-mean-square (RMS) minus 1 standard deviation of the energy gaps and root-mean-square (RMS) plus 1 standard deviation of the spin-orbit couplings between each pair of singlet and triplet.

| Tn | Sn | job11 | job14 | job36 | job54 | job66 | job67 | job7 | job87 | job90 | average |
|---|---|---|---|---|---|---|---|---|---|---|---|
| 0 | 0 | $2.372\times10^{-3}$ | $1.846\times10^{-3}$ | $2.298\times10^{-3}$ | $1.696\times10^{-3}$ | $2.179\times10^{-3}$ | $2.560\times10^{-3}$ | $3.648\times10^{-3}$ | $2.140\times10^{-3}$ | $1.912\times10^{-3}$ | $2.294\times10^{-3}$ |
| 1 | 0 | $2.580\times10^{-2}$ | $1.532\times10^{-2}$ | $1.589\times10^{-2}$ | $2.474\times10^{-2}$ | $2.019\times10^{-2}$ | $1.605\times10^{-2}$ | $2.620\times10^{-2}$ | $1.725\times10^{-2}$ | $1.458\times10^{-2}$ | $1.956\times10^{-2}$ |
| 2 | 0 | $1.226\times10^{-2}$ | $1.819\times10^{-2}$ | $1.113\times10^{-2}$ | $1.501\times10^{-2}$ | $1.406\times10^{-2}$ | $1.229\times10^{-2}$ | $1.892\times10^{-2}$ | $1.235\times10^{-2}$ | $1.027\times10^{-2}$ | $1.383\times10^{-2}$ |
| 3 | 0 | $7.936\times10^{-3}$ | $6.822\times10^{-3}$ | $5.816\times10^{-3}$ | $7.541\times10^{-3}$ | $6.085\times10^{-3}$ | $5.831\times10^{-3}$ | $7.519\times10^{-3}$ | $6.624\times10^{-3}$ | $3.527\times10^{-3}$ | $6.411\times10^{-3}$ |
| 4 | 0 | $5.347\times10^{-3}$ | $4.594\times10^{-3}$ | $3.948\times10^{-3}$ | $4.770\times10^{-3}$ | $4.219\times10^{-3}$ | $3.773\times10^{-3}$ | $5.697\times10^{-3}$ | $4.392\times10^{-3}$ | $2.570\times10^{-3}$ | $4.368\times10^{-3}$ |
| 0 | 1 | $5.877\times10^{-3}$ | $4.245\times10^{-3}$ | $1.153\times10^{-2}$ | $5.598\times10^{-3}$ | $1.100\times10^{-2}$ | $9.994\times10^{-3}$ | $9.625\times10^{-3}$ | $9.351\times10^{-3}$ | $5.433\times10^{-3}$ | $8.072\times10^{-3}$ |
| 1 | 1 | $2.750\times10^{-3}$ | $1.103\times10^{-3}$ | $1.156\times10^{-3}$ | $1.602\times10^{-3}$ | $1.701\times10^{-3}$ | $1.464\times10^{-3}$ | $1.854\times10^{-3}$ | $1.627\times10^{-3}$ | $1.095\times10^{-3}$ | $1.595\times10^{-3}$ |
| 2 | 1 | $5.944\times10^{-3}$ | $2.432\times10^{-3}$ | $5.399\times10^{-3}$ | $3.940\times10^{-3}$ | $4.642\times10^{-3}$ | $4.954\times10^{-3}$ | $6.592\times10^{-3}$ | $4.203\times10^{-3}$ | $4.339\times10^{-3}$ | $4.716\times10^{-3}$ |
| 3 | 1 | $1.577\times10^{-3}$ | $8.154\times10^{-4}$ | $2.530\times10^{-3}$ | $1.569\times10^{-3}$ | $2.258\times10^{-3}$ | $2.337\times10^{-3}$ | $1.652\times10^{-3}$ | $2.653\times10^{-3}$ | $1.018\times10^{-3}$ | $1.823\times10^{-3}$ |
| 4 | 1 | $1.963\times10^{-3}$ | $1.151\times10^{-3}$ | $1.845\times10^{-3}$ | $1.788\times10^{-3}$ | $1.908\times10^{-3}$ | $1.398\times10^{-3}$ | $1.258\times10^{-3}$ | $1.821\times10^{-3}$ | $7.554\times10^{-4}$ | $1.543\times10^{-3}$ |
| 0 | 2 | $2.860\times10^{-2}$ | $3.812\times10^{-2}$ | $1.743\times10^{-2}$ | $3.191\times10^{-2}$ | $2.532\times10^{-2}$ | $1.995\times10^{-2}$ | $3.465\times10^{-2}$ | $2.040\times10^{-2}$ | $1.569\times10^{-2}$ | $2.579\times10^{-2}$ |
| 1 | 2 | $5.358\times10^{-3}$ | $3.326\times10^{-3}$ | $7.405\times10^{-3}$ | $4.603\times10^{-3}$ | $7.471\times10^{-3}$ | $6.947\times10^{-3}$ | $9.672\times10^{-3}$ | $6.818\times10^{-3}$ | $4.405\times10^{-3}$ | $6.223\times10^{-3}$ |
| 2 | 2 | $3.160\times10^{-3}$ | $4.263\times10^{-3}$ | $2.743\times10^{-3}$ | $4.021\times10^{-3}$ | $2.918\times10^{-3}$ | $2.453\times10^{-3}$ | $4.422\times10^{-3}$ | $3.042\times10^{-3}$ | $1.133\times10^{-3}$ | $3.128\times10^{-3}$ |
| 3 | 2 | $8.105\times10^{-4}$ | $1.432\times10^{-3}$ | $1.262\times10^{-3}$ | $1.786\times10^{-3}$ | $1.524\times10^{-3}$ | $1.175\times10^{-3}$ | $1.411\times10^{-3}$ | $1.577\times10^{-3}$ | $6.822\times10^{-4}$ | $1.295\times10^{-3}$ |
| 4 | 2 | $5.521\times10^{-3}$ | $7.074\times10^{-3}$ | $3.468\times10^{-3}$ | $6.022\times10^{-3}$ | $4.561\times10^{-3}$ | $3.634\times10^{-3}$ | $6.730\times10^{-3}$ | $3.727\times10^{-3}$ | $2.798\times10^{-3}$ | $4.837\times10^{-3}$ |
| 0 | 3 | $3.011\times10^{-3}$ | $2.342\times10^{-3}$ | $2.690\times10^{-3}$ | $2.988\times10^{-3}$ | $3.113\times10^{-3}$ | $2.727\times10^{-3}$ | $3.446\times10^{-3}$ | $3.121\times10^{-3}$ | $2.315\times10^{-3}$ | $2.862\times10^{-3}$ |
| 1 | 3 | $8.812\times10^{-3}$ | $5.076\times10^{-3}$ | $1.002\times10^{-2}$ | $8.229\times10^{-3}$ | $1.069\times10^{-2}$ | $8.070\times10^{-3}$ | $1.150\times10^{-2}$ | $8.296\times10^{-3}$ | $4.987\times10^{-3}$ | $8.409\times10^{-3}$ |
| 2 | 3 | $1.088\times10^{-3}$ | $1.940\times10^{-3}$ | $4.059\times10^{-3}$ | $1.702\times10^{-3}$ | $4.942\times10^{-3}$ | $3.533\times10^{-3}$ | $2.844\times10^{-3}$ | $2.915\times10^{-3}$ | $1.631\times10^{-3}$ | $2.739\times10^{-3}$ |
| 3 | 3 | $1.965\times10^{-3}$ | $6.253\times10^{-4}$ | $4.211\times10^{-3}$ | $1.516\times10^{-3}$ | $3.868\times10^{-3}$ | $2.853\times10^{-3}$ | $2.850\times10^{-3}$ | $3.281\times10^{-3}$ | $1.048\times10^{-3}$ | $2.469\times10^{-3}$ |
| 4 | 3 | $1.841\times10^{-3}$ | $8.608\times10^{-4}$ | $1.694\times10^{-3}$ | $1.233\times10^{-3}$ | $1.718\times10^{-3}$ | $1.340\times10^{-3}$ | $1.639\times10^{-3}$ | $1.571\times10^{-3}$ | $9.559\times10^{-4}$ | $1.428\times10^{-3}$ |
| 0 | 4 | $2.526\times10^{-3}$ | $2.098\times10^{-3}$ | $2.760\times10^{-3}$ | $2.229\times10^{-3}$ | $3.062\times10^{-3}$ | $2.471\times10^{-3}$ | $3.457\times10^{-3}$ | $2.435\times10^{-3}$ | $2.000\times10^{-3}$ | $2.560\times10^{-3}$ |
| 1 | 4 | $2.277\times10^{-2}$ | $2.444\times10^{-2}$ | $1.472\times10^{-2}$ | $2.504\times10^{-2}$ | $2.140\times10^{-2}$ | $1.406\times10^{-2}$ | $1.926\times10^{-2}$ | $1.578\times10^{-2}$ | $1.104\times10^{-2}$ | $1.872\times10^{-2}$ |
| 2 | 4 | $9.648\times10^{-3}$ | $2.308\times10^{-2}$ | $1.212\times10^{-2}$ | $1.629\times10^{-2}$ | $1.729\times10^{-2}$ | $1.452\times10^{-2}$ | $1.705\times10^{-2}$ | $1.319\times10^{-2}$ | $7.742\times10^{-3}$ | $1.455\times10^{-2}$ |
| 3 | 4 | $2.777\times10^{-3}$ | $1.663\times10^{-3}$ | $6.646\times10^{-3}$ | $2.295\times10^{-3}$ | $7.276\times10^{-3}$ | $5.599\times10^{-3}$ | $3.988\times10^{-3}$ | $5.397\times10^{-3}$ | $1.872\times10^{-3}$ | $4.168\times10^{-3}$ |
| 4 | 4 | $5.294\times10^{-3}$ | $4.414\times10^{-3}$ | $5.613\times10^{-3}$ | $4.519\times10^{-3}$ | $5.911\times10^{-3}$ | $4.899\times10^{-3}$ | $6.402\times10^{-3}$ | $5.424\times10^{-3}$ | $2.694\times10^{-3}$ | $5.019\times10^{-3}$ |
| 0 | 5 | $2.366\times10^{-3}$ | $3.609\times10^{-3}$ | $3.281\times10^{-3}$ | $3.306\times10^{-3}$ | $3.828\times10^{-3}$ | $3.322\times10^{-3}$ | $3.553\times10^{-3}$ | $3.453\times10^{-3}$ | $1.963\times10^{-3}$ | $3.187\times10^{-3}$ |
| 1 | 5 | $1.971\times10^{-2}$ | $1.390\times10^{-2}$ | $1.219\times10^{-2}$ | $1.880\times10^{-2}$ | $1.766\times10^{-2}$ | $1.258\times10^{-2}$ | $1.954\times10^{-2}$ | $1.334\times10^{-2}$ | $8.642\times10^{-3}$ | $1.515\times10^{-2}$ |
| 2 | 5 | $1.659\times10^{-2}$ | $4.693\times10^{-2}$ | $2.186\times10^{-2}$ | $3.847\times10^{-2}$ | $3.014\times10^{-2}$ | $2.370\times10^{-2}$ | $3.840\times10^{-2}$ | $2.535\times10^{-2}$ | $1.491\times10^{-2}$ | $2.849\times10^{-2}$ |
| 3 | 5 | $3.670\times10^{-3}$ | $4.571\times10^{-3}$ | $8.666\times10^{-3}$ | $6.904\times10^{-3}$ | $9.067\times10^{-3}$ | $8.545\times10^{-3}$ | $5.821\times10^{-3}$ | $9.654\times10^{-3}$ | $3.420\times10^{-3}$ | $6.702\times10^{-3}$ |
| 4 | 5 | $8.257\times10^{-3}$ | $1.419\times10^{-2}$ | $9.807\times10^{-3}$ | $1.116\times10^{-2}$ | $1.044\times10^{-2}$ | $9.570\times10^{-3}$ | $1.194\times10^{-2}$ | $1.102\times10^{-2}$ | $3.668\times10^{-3}$ | $1.001\times10^{-2}$ |

TABLE SV: Landau-Zener probabilities calculated using root-mean-square (RMS) plus 1 standard deviation of the energy gaps and root-mean-square (RMS) minus 1 standard deviation of the spin-orbit couplings between each pair of singlet and triplet.

| Tn | Sn | job11 | job14 | job36 | job54 | job66 | job67 | job7 | job87 | job90 | average |
|---|---|---|---|---|---|---|---|---|---|---|---|
| 0 | 0 | $3.088\times10^{-5}$ | $3.162\times10^{-5}$ | $1.403\times10^{-5}$ | $1.848\times10^{-5}$ | $1.298\times10^{-5}$ | $1.348\times10^{-5}$ | $2.421\times10^{-5}$ | $1.657\times10^{-5}$ | $9.870\times10^{-6}$ | $1.912\times10^{-5}$ |
| 1 | 0 | $6.137\times10^{-4}$ | $1.283\times10^{-3}$ | $2.267\times10^{-4}$ | $8.485\times10^{-4}$ | $3.034\times10^{-4}$ | $2.103\times10^{-4}$ | $5.051\times10^{-4}$ | $2.480\times10^{-4}$ | $8.173\times10^{-5}$ | $4.800\times10^{-4}$ |
| 2 | 0 | $4.046\times10^{-4}$ | $1.287\times10^{-3}$ | $3.263\times10^{-4}$ | $7.686\times10^{-4}$ | $4.410\times10^{-4}$ | $3.403\times10^{-4}$ | $7.591\times10^{-4}$ | $3.313\times10^{-4}$ | $8.037\times10^{-5}$ | $5.265\times10^{-4}$ |
| 3 | 0 | $9.972\times10^{-5}$ | $1.347\times10^{-4}$ | $6.258\times10^{-5}$ | $1.224\times10^{-4}$ | $7.462\times10^{-5}$ | $6.430\times10^{-5}$ | $7.792\times10^{-5}$ | $6.361\times10^{-5}$ | $1.313\times10^{-5}$ | $7.922\times10^{-5}$ |
| 4 | 0 | $1.221\times10^{-4}$ | $1.852\times10^{-4}$ | $5.654\times10^{-5}$ | $1.448\times10^{-4}$ | $6.851\times10^{-5}$ | $5.695\times10^{-5}$ | $1.108\times10^{-4}$ | $6.258\times10^{-5}$ | $1.144\times10^{-5}$ | $9.099\times10^{-5}$ |
| 0 | 1 | $1.055\times10^{-4}$ | $1.382\times10^{-4}$ | $1.701\times10^{-4}$ | $1.225\times10^{-4}$ | $1.425\times10^{-4}$ | $1.304\times10^{-4}$ | $1.216\times10^{-4}$ | $1.145\times10^{-4}$ | $2.899\times10^{-5}$ | $1.194\times10^{-4}$ |
| 1 | 1 | $1.066\times10^{-5}$ | $8.780\times10^{-6}$ | $4.520\times10^{-6}$ | $8.012\times10^{-6}$ | $4.655\times10^{-6}$ | $4.486\times10^{-6}$ | $5.036\times10^{-6}$ | $5.171\times10^{-6}$ | $1.664\times10^{-6}$ | $5.887\times10^{-6}$ |
| 2 | 1 | $6.302\times10^{-5}$ | $1.157\times10^{-4}$ | $4.867\times10^{-5}$ | $8.727\times10^{-5}$ | $5.891\times10^{-5}$ | $4.737\times10^{-5}$ | $8.555\times10^{-5}$ | $4.159\times10^{-5}$ | $1.046\times10^{-5}$ | $6.206\times10^{-5}$ |
| 3 | 1 | $2.127\times10^{-5}$ | $1.764\times10^{-5}$ | $1.403\times10^{-5}$ | $2.142\times10^{-5}$ | $1.430\times10^{-5}$ | $1.079\times10^{-5}$ | $1.401\times10^{-5}$ | $1.477\times10^{-5}$ | $3.891\times10^{-6}$ | $1.468\times10^{-5}$ |
| 4 | 1 | $9.050\times10^{-6}$ | $1.008\times10^{-5}$ | $9.031\times10^{-6}$ | $1.141\times10^{-5}$ | $8.645\times10^{-6}$ | $8.081\times10^{-6}$ | $7.841\times10^{-6}$ | $8.757\times10^{-6}$ | $2.103\times10^{-6}$ | $8.333\times10^{-6}$ |
| 0 | 2 | $8.487\times10^{-4}$ | $2.799\times10^{-3}$ | $4.161\times10^{-4}$ | $1.732\times10^{-3}$ | $6.239\times10^{-4}$ | $4.359\times10^{-4}$ | $1.266\times10^{-3}$ | $4.437\times10^{-4}$ | $7.188\times10^{-5}$ | $9.597\times10^{-4}$ |
| 1 | 2 | $9.159\times10^{-5}$ | $2.060\times10^{-4}$ | $5.757\times10^{-5}$ | $1.275\times10^{-4}$ | $7.169\times10^{-5}$ | $5.843\times10^{-5}$ | $1.120\times10^{-4}$ | $4.955\times10^{-5}$ | $9.836\times10^{-6}$ | $8.712\times10^{-5}$ |
| 2 | 2 | $1.284\times10^{-5}$ | $2.022\times10^{-5}$ | $7.015\times10^{-6}$ | $1.613\times10^{-5}$ | $7.765\times10^{-6}$ | $6.508\times10^{-6}$ | $8.948\times10^{-6}$ | $7.473\times10^{-6}$ | 8.483E-07 | $9.750\times10^{-6}$ |
| 3 | 2 | $7.036\times10^{-6}$ | $1.738\times10^{-5}$ | $9.421\times10^{-6}$ | $1.723\times10^{-5}$ | $1.080\times10^{-5}$ | $8.634\times10^{-6}$ | $1.246\times10^{-5}$ | $1.045\times10^{-5}$ | $1.572\times10^{-6}$ | $1.055\times10^{-5}$ |
| 4 | 2 | $1.245\times10^{-4}$ | $3.562\times10^{-4}$ | $4.193\times10^{-5}$ | $2.098\times10^{-4}$ | $6.684\times10^{-5}$ | $4.957\times10^{-5}$ | $1.712\times10^{-4}$ | $5.272\times10^{-5}$ | $8.084\times10^{-6}$ | $1.201\times10^{-4}$ |
| 0 | 3 | $1.824\times10^{-5}$ | $1.098\times10^{-5}$ | $1.980\times10^{-5}$ | $1.733\times10^{-5}$ | $1.952\times10^{-5}$ | $1.375\times10^{-5}$ | $1.212\times10^{-5}$ | $2.184\times10^{-5}$ | $3.419\times10^{-6}$ | $1.522\times10^{-5}$ |
| 1 | 3 | $2.706\times10^{-5}$ | $3.084\times10^{-5}$ | $2.281\times10^{-5}$ | $2.836\times10^{-5}$ | $2.207\times10^{-5}$ | $1.665\times10^{-5}$ | $2.164\times10^{-5}$ | $2.049\times10^{-5}$ | $2.613\times10^{-6}$ | $2.139\times10^{-5}$ |
| 2 | 3 | $7.467\times10^{-6}$ | $2.729\times10^{-5}$ | $1.579\times10^{-5}$ | $2.280\times10^{-5}$ | $1.811\times10^{-5}$ | $1.249\times10^{-5}$ | $1.804\times10^{-5}$ | $1.500\times10^{-5}$ | $1.751\times10^{-6}$ | $1.542\times10^{-5}$ |
| 3 | 3 | $2.153\times10^{-6}$ | $4.926\times10^{-6}$ | $4.017\times10^{-6}$ | $4.351\times10^{-6}$ | $3.304\times10^{-6}$ | $2.450\times10^{-6}$ | $2.565\times10^{-6}$ | $3.222\times10^{-6}$ | 3.806E-07 | $3.041\times10^{-6}$ |
| 4 | 3 | $9.378\times10^{-6}$ | $2.470\times10^{-5}$ | $7.871\times10^{-6}$ | $1.614\times10^{-5}$ | $8.620\times10^{-6}$ | $7.097\times10^{-6}$ | $1.189\times10^{-5}$ | $8.130\times10^{-6}$ | $1.085\times10^{-6}$ | $1.055\times10^{-5}$ |
| 0 | 4 | $4.687\times10^{-5}$ | $6.267\times10^{-5}$ | $3.644\times10^{-5}$ | $5.099\times10^{-5}$ | $4.182\times10^{-5}$ | $2.855\times10^{-5}$ | $4.705\times10^{-5}$ | $3.303\times10^{-5}$ | $5.622\times10^{-6}$ | $3.923\times10^{-5}$ |
| 1 | 4 | $1.760\times10^{-4}$ | $2.514\times10^{-4}$ | $6.223\times10^{-5}$ | $2.070\times10^{-4}$ | $8.646\times10^{-5}$ | $5.981\times10^{-5}$ | $1.240\times10^{-4}$ | $6.390\times10^{-5}$ | $1.089\times10^{-5}$ | $1.157\times10^{-4}$ |
| 2 | 4 | $7.108\times10^{-5}$ | $2.563\times10^{-4}$ | $7.296\times10^{-5}$ | $1.494\times10^{-4}$ | $1.075\times10^{-4}$ | $8.094\times10^{-5}$ | $1.385\times10^{-4}$ | $7.033\times10^{-5}$ | $6.964\times10^{-6}$ | $1.060\times10^{-4}$ |
| 3 | 4 | $1.469\times10^{-5}$ | $2.266\times10^{-5}$ | $1.378\times10^{-5}$ | $2.305\times10^{-5}$ | $1.398\times10^{-5}$ | $1.110\times10^{-5}$ | $1.385\times10^{-5}$ | $1.288\times10^{-5}$ | $1.176\times10^{-6}$ | $1.413\times10^{-5}$ |
| 4 | 4 | $4.085\times10^{-5}$ | $5.272\times10^{-5}$ | $1.710\times10^{-5}$ | $4.331\times10^{-5}$ | $2.202\times10^{-5}$ | $1.789\times10^{-5}$ | $3.779\times10^{-5}$ | $2.191\times10^{-5}$ | $2.344\times10^{-6}$ | $2.844\times10^{-5}$ |
| 0 | 5 | $3.850\times10^{-5}$ | $5.135\times10^{-5}$ | $4.122\times10^{-5}$ | $4.051\times10^{-5}$ | $4.026\times10^{-5}$ | $3.142\times10^{-5}$ | $4.221\times10^{-5}$ | $3.765\times10^{-5}$ | $6.860\times10^{-6}$ | $3.666\times10^{-5}$ |
| 1 | 5 | $8.250\times10^{-5}$ | $1.396\times10^{-4}$ | $4.573\times10^{-5}$ | $1.273\times10^{-4}$ | $6.013\times10^{-5}$ | $3.734\times10^{-5}$ | $6.420\times10^{-5}$ | $4.186\times10^{-5}$ | $5.814\times10^{-6}$ | $6.717\times10^{-5}$ |
| 2 | 5 | $1.331\times10^{-4}$ | $5.830\times10^{-4}$ | $1.350\times10^{-4}$ | $3.885\times10^{-4}$ | $2.085\times10^{-4}$ | $1.498\times10^{-4}$ | $3.387\times10^{-4}$ | $1.500\times10^{-4}$ | $1.611\times10^{-5}$ | $2.336\times10^{-4}$ |
| 3 | 5 | $1.738\times10^{-5}$ | $2.027\times10^{-5}$ | $2.102\times10^{-5}$ | $2.715\times10^{-5}$ | $1.998\times10^{-5}$ | $1.529\times10^{-5}$ | $1.646\times10^{-5}$ | $2.204\times10^{-5}$ | $1.612\times10^{-6}$ | $1.791\times10^{-5}$ |
| 4 | 5 | $3.650\times10^{-5}$ | $5.564\times10^{-5}$ | $2.381\times10^{-5}$ | $4.920\times10^{-5}$ | $2.682\times10^{-5}$ | $2.172\times10^{-5}$ | $3.377\times10^{-5}$ | $2.844\times10^{-5}$ | $2.151\times10^{-6}$ | $3.090\times10^{-5}$ |
